# Supplementary material for: Measuring Policy Distance for Multi-Agent Reinforcement Learning
Source: arXiv:2401.11257 source file (2024-01-28)
Supplement: Supplementary file 1 [file Appendices.pdf]

# APPENDICES

# 1 THEORIES

## 1.1 Multi-Agent Policy Distance

The policy distance between two agents following MPD in Section 3.3 can be computed as follows:

$$d_{ij} = \int_{O' \subseteq O_P} W\left[p_i(z|o), p_j(z|o)\right] do, \tag{1}$$

where $p_i(z|o) = f_\phi[z|\pi_i(a|o), o]$ denotes the latent distribution of agent $i$ under observation $o$, $W$ denotes a distribution distance, $O'$ is a subset of the observation space $O_P$. The integral symbol in the above formula is just a concept that represents traversing the entire observation space (thus applicable to discrete observation spaces). It can be proven that when $W$ satisfies Prop.1-5 in Section 3.1, MPD also satisfies Prop.1-5.

*1) Proof of Symmetry:*

$$d_{ij} = \int_{O'} W\left[p_i(z|o), p_j(z|o)\right] do = \int_{O'} W\left[p_j(z|o), p_i(z|o)\right] do = d_{ji}. \tag{2}$$

*2) Proof of Non-negativity:*

$$d_{ij} = \int_{O'} W\left[p_i(z|o), p_j(z|o)\right] do \geq \int_{O'} 0 \cdot do = 0. \tag{3}$$

*3) Proof of Identicals of indiscernibility (necessary conditions):*

$$\begin{aligned} d_{ij}|_{\pi_i=\pi_j} &= \int_{O'} W\left[p_i(z|o), p_j(z|o)\right] do = \int_{O'} W\left[f_\phi[z|\pi_i(a|o), o], f_\phi[z|\pi_j(a|o), o]\right] do \\ &= \int_{O'} W\left[f_\phi[z|\pi_i(a|o), o], f_\phi[z|\pi_i(a|o), o]\right] do = \int_{O'} 0 \cdot do = 0. \end{aligned} \tag{4}$$

*4) Proof of Identicals of indiscernibility (sufficient conditions):*

$$d_{ij} = 0 \xrightarrow{\text{Prop.2}} W\left[p_i(z|o), p_j(z|o)\right] = 0, \forall o \in O' \xrightarrow{\text{Prop.2 of } W} f_\phi[z|\pi_i(a|o), o] = f_\phi[z|\pi_j(a|o), o], \forall o \in O'. \tag{5}$$

*5) Proof of Triangle inequality:*

$$\begin{aligned} d_{ij} &= \int_{O'} W\left[p_i(z|o), p_j(z|o)\right] do \leq \int_{O'} \left(W\left[p_i(z|o), p_k(z|o)\right] + W\left[p_k(z|o), p_j(z|o)\right]\right) do \\ &= \int_{O'} W\left[p_i(z|o), p_k(z|o)\right] do + \int_{O'} W\left[p_k(z|o), p_j(z|o)\right] do = d_{ik} + d_{kj}. \end{aligned} \tag{6}$$

In the *proof of the sufficient conditions for the identicals of indiscernibility*, the condition $d_{ij} = 0$ only guarantees that $\forall o \in O'$, $f_\phi[z|\pi_i(a|o), o] = f_\phi[z|\pi_j(a|o), o]$, but it does not imply that $\pi_i = \pi_j$. An example would be $f_\phi$ mapping all inputs to the same distribution, but our reconstruction loss can prevent such things from happening .

In practical applications, it is intractable to compute the policy distance by traversing the entire observation space. In fact, the set of observations involved in multi-agent tasks (determined by the initial state and the state transition function) may only constitute a small portion of the observation space. Hence, we focus only on the relevant observations $o \in O'$, specifically those that occur during the actual tasks. In experiments, we use Monte Carlo sampling to estimate the integral and employ multi-rollout to reduce estimation variance. $O'$ in Eq. 1 actually represents the set of all valid observations in the observation space. In certain scenarios, there may be persistent invalid observations, such as in the SMAC where observations are set to an zero-vector after an agent's death, even while the environment remains active. Including these zero vectors in the sampling process and performing averaging computations would result in significant errors, as $O'$ excludes such invalid observations.

## 1.2 Proofs of ELBO in Customized Representation Learning

To optimize the likelihood $\log p(\boldsymbol{c}|o)$ corresponding to the prior distribution of customized feature $\boldsymbol{c}$, an Evidence Lower Bound (ELBO) of the likelihood can be derived as follows:

$$
\begin{aligned}
\log p(\mathbf{c}|o) &= \log \int p(\mathbf{c}, z|o)dz & \text{(a)} \\
&= \log \int \frac{p(\mathbf{c}, z|o) f_{\phi^c}[z|\pi_i(a|o), o]}{f_{\phi^c}[z|\pi_i(a|o), o]} dz & \text{(b)} \\
&= \log \mathbb{E}_{f_{\phi^c}[z|\pi_i(a|o),o]} \left[ \frac{p(\mathbf{c}, z|o)}{f_{\phi^c}[z|\pi_i(a|o), o]} \right] & \text{(c)} \\
&\geq \mathbb{E}_{f_{\phi^c}[z|\pi_i(a|o),o]} \left[ \log \frac{p(\mathbf{c}, z|o)}{f_{\phi^c}[z|\pi_i(a|o), o]} \right], & \text{(d)}
\end{aligned}
\tag{7}
$$

where $f_{\phi^c}[z|\pi_i(a|o), o]$ represents the posterior probability distribution of the latent variable generated by the encoder, and $p(\mathbf{c}, z|o)$ denotes a joint probability distribution concerning the customized feature and latent variable, conditioned on $o$. Throughout the derivation of the formula, (a) employs the properties of the joint probability distribution, (b) multiplies both numerator and denominator by $f_{\phi^c}[z|\pi_i(a|o), o]$, (c) applies the definition of mathematical expectation, and (d) invokes the Jensen's inequality.

Considering that the ELBO includes an unknown joint probability distribution, we can further decompose it by using the posterior probability distributions from the encoder and decoder:

$$
\begin{aligned}
&\mathbb{E}_{f_{\phi^c}[z|\pi_i(a|o),o]} \left[ \log \frac{p(\mathbf{c}, z|o)}{f_{\phi^c}[z|\pi_i(a|o), o]} \right] \\
&= \mathbb{E}_{f_{\phi^c}[z|\pi_i(a|o),o]} \left[ \log \frac{g_\omega(\mathbf{c}|z, o) p(z|o)}{f_{\phi^c}[z|\pi_i(a|o), o]} \right] & \text{(a)} \\
&= \mathbb{E}_{f_{\phi^c}[z|\pi_i(a|o),o]} [\log g_\omega(\mathbf{c}|z, o)] \\
&\quad + \mathbb{E}_{f_{\phi^c}[z|\pi_i(a|o),o]} \left[ \log \frac{p(z|o)}{f_{\phi^c}[z|\pi_i(a|o), o]} \right] & \text{(b)} \\
&= \underbrace{\mathbb{E}_{f_{\phi^c}[z|\pi_i(a|o),o]} [\log g_\omega(\mathbf{c}|z, o)]}_{\text{reconstruction term}} - \underbrace{D_{\mathrm{KL}} \left( f_{\phi^c}[z|\pi_i(a|o), o] \| p(z|o) \right)}_{\text{prior matching term}}, & \text{(c)}
\end{aligned}
\tag{8}
$$

where $f_{\phi^c}[z|\pi_i(a|o), o]$ and $g_\omega(\mathbf{c}|z, o)$ are the posteriors from the encoder and decoder, respectively. The conditional joint probability distribution $p(\mathbf{c}, z|o)$ is a imaginary construct in mathematical terms and lacks practical significance. It can be formulated using the probability chain rule, constructed from the posterior distribution of the customized feature and the prior distribution of the latent variable (step (a)). Step (b) decomposes the expectation, and step (c) applies the definition of the KL divergence.

Thus, the ELBO can be decomposed into a reconstruction term of the customized feature, and a prior matching term of the posterior and the prior. By maximizing the ELBO, the reconstruction likelihood can be maximized while minimizing the KL divergence between the posterior and the prior.

## 2 ALGORITHM OF DYNAMIC PARAMETER SHARING

The basic idea of MDPS can be summarized as: giving a fusion threshold $\epsilon_1$ and a division threshold $\epsilon_2$, when $d_{ij} < \epsilon_1$, the agents attempt to fuse part of their network parameters. When $d_{ij} > \epsilon_2$ and the agents have shared network components, they will undergo policy division. If $\epsilon_1 \leq d_{ij} \leq \epsilon_2$, agents maintain their strategy independence.

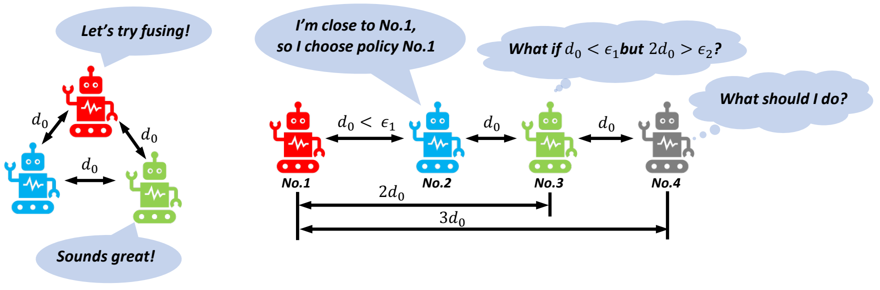


**Figure 1: Parameter sharing issues in multiple agent cases.**

When addressing parameter sharing among multiple agents, the interrelationship between fusion and division thresholds should be considered carefully. Fig. 1 (left) depicts a normal case of parameter sharing among 3 agents, where the policy distance between each pair of agents is $d_0 < \epsilon_1$. Therefore, they can select a *public* policy for fusion. Since the agents are still in training and it cannot be asserted which agent has the optimal policy (especially considering their policies are quit close), any of these polices can be chosen as the public one. However, what if the policy distances between the multiple agents are not equal? According to the triangle inequality property of strategy distances, the most extreme case would be two agents with a distance of $d_0$ and the other two agents with a distance of $2d_0$, as shown in Fig.1 (right). In this case, contradictions may arise between policy fusion and division.

The first contradiction arises when $d_0 < \epsilon_1$ while $2d_0 > \epsilon_2$. We use $(i,j)$ to denote the pair of agent $i$ and $j$. In this case, policy fusion is required between (1,2) and (2,3), but a policy division is needed between (1,3), resulting in a conflict. To avoid this situation, we let $\epsilon_2 \geq 2\epsilon_1$, so $2d_0$ will be always smaller than $\epsilon_2$ (in our experiments, we directly set $\epsilon_2 = 2\epsilon_1$ to reduce the number of hyperparameters). The second contradiction arises when $d_0 < \epsilon_1$ while $2d_0 > \epsilon_1$. In this case, if (1,2) and (2,3) both choose policy NO.2 as the public policy for fusion, according to the above rules, (1,3) should maintain their policy independence, leading to another contradiction. To address this issue, MAPS examines the policy distance between agents in ascending order of their indices. When the policy distance between agent $i$ and agent $j (i < j)$ is smaller than $\epsilon_1$, MAPS additionally check the distance between agent $i$'s new policy (if any, denoted as $Net^N(i)$) and that of agent $j$. If this distance is still smaller than $\epsilon_1$, MAPS fuses $j$'s policy with $Net^N(i)$, else with agent $i$'s original policy, denoted as $Net^O(i)$. This approach ensures more agents' policies are fused into the networks with lower indices, thereby improving sampling efficiency and avoiding possible conflicts. The corresponding algorithm is presented in Algorithm 1. In Algorithm 1, we only list the fusion and division operations for the front layer and back layer of the nerual network (which is the simplest case), to provide a clearer explanation of the algorithm's principles.

**Algorithm 1** Dynamic Parameter Sharing based on MPD

**Input:** MPD matrix $D$, front-layer indices $FL$, back-layer indices $BL$, fusion threshold $\epsilon_1$
Division threshold $\epsilon_2 \leftarrow 2\epsilon_1$.
**for** agent $i \in \{1, \cdots, n\}$ **do**
  **for** agent $j \in \{i+1, \cdots, n\}$ **do**
    **if** $FL[i] \neq FL[j]$ **then**
      **if** $D(i,j) < \epsilon_1$ **then**
        *Fuse the front-layer:*
        **if** $D(FL[i], j) < \epsilon 1$ **then**
          $FL[j] \leftarrow FL[i]$
        **else**
          $FL[j] \leftarrow i$
        **end if**
      **end if**
    **else**
      **if** $D(i,j) < \epsilon_1$ **then**
        *Fuse the back-layer:*
        **if** $D(FL[i], j) < \epsilon 1$ **then**
          $FL[j] \leftarrow FL[i]$
        **else**
          $FL[j] \leftarrow i$
        **end if**
      **else if** $D(i,j) > \epsilon_2$ **then**
        *Divide the front-layer:*
      $DL[j] \leftarrow j$, copy the parameters of $DL[j]$ from $DL[i]$
      **end if**
    **end if**
  **end for**
**end for**

## 3 EXPERIMENTAL DETAILS

### 3.1 Performance of Vanilla methods of measuring policy distance

We conduct an experiment in the original multi-agent spread scenario to illustrate the limitations of directly measuring the action distributions. Fig. 2 depicts the reward curve and average policy distance curves of agents in this scenario, where agents are required to spread towards corresponding landmarks, and all agents perform discret actions. During the training process, the parameters of each agent's network are

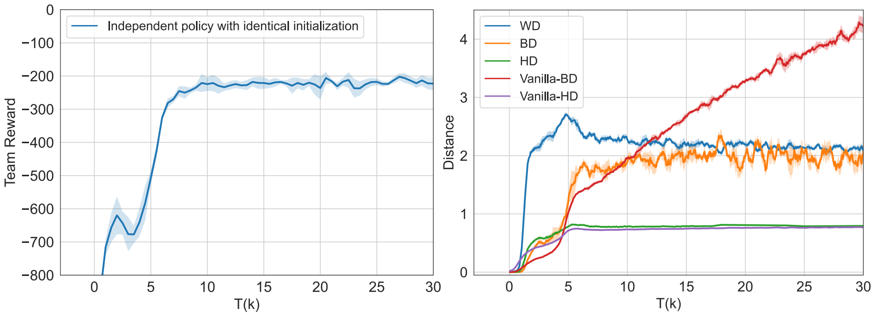


(a) Reward Curve (b) Distance Curves

**Figure 2: The reward curve and average policy distance curves in a naive multi-agent spread environment.**

independent but initialized as the same. Here, *WD*, *BD*, and *HD* denote the distance curves corresponding to our proposed method using Wasserstein, Bhattacharyya, and Hellinger distances respectively. *Vanilla-BD* and *Vanilla-HD* represent the curves when directly using the action distribution for measurements. The absence of the *Vanilla-WD* curve is due to the inability to calculate the W-distance of agent policies without a known discrete action cost matrix (because the indices of actions are meaningless).

As shown in Figure 1, agents with independent parameters and identical initialization gradually evolve distinct policies. This is evident from the initial increase in the distance curves. When agents' policies tend to converge, the curves of our method also stabilizes, indicating the diversity level of the entire multi-agent system becomes steady. However, the distance curves of vanilla method keep increasing during training (even reaching *inf* in our experiments). This implies that the vanilla method can only superficially characterize the differences in agent policies based on input-output, without truly capturing a higher level differences between policies.

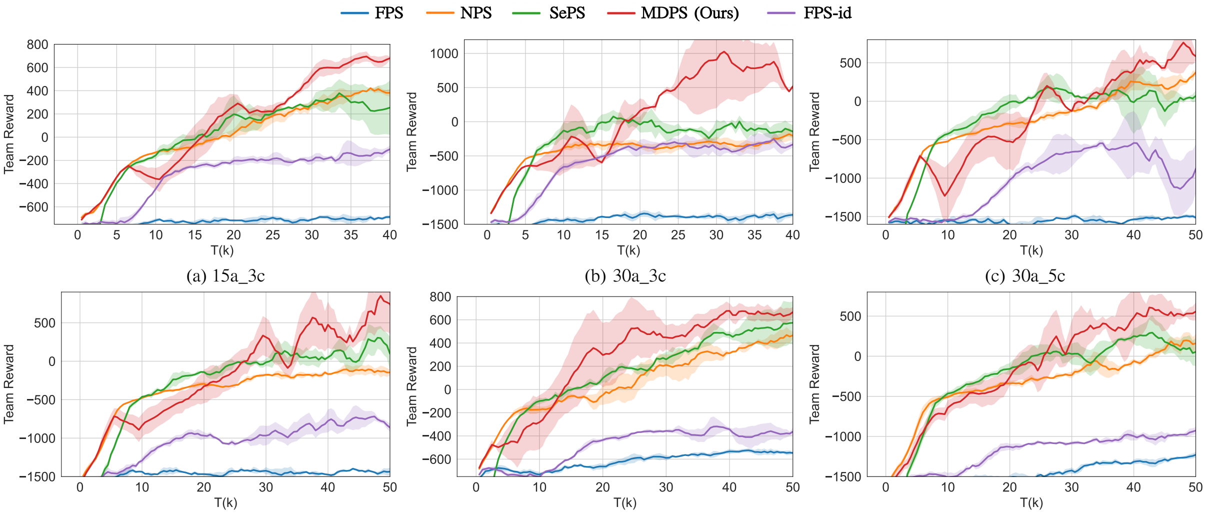


(a) 15a_3c (b) 30a_3c (c) 30a_5c

(d) 30a_5c_super (e) 15a_3c_shuffle (f) 30a_5c_ shuffle

**Figure 3: Comparisons between MDPS and baselines in 6 harder multi-agent spread scenarios.**

## 3.2 Experimental Settings

For all experiments, the methods about parameter sharing are conducted using actor-critic with a learning rate of $3 \times 10^{-4}$, discount factor $\gamma$ of 0.99, entropy loss coefficient of 0.01 and value loss coefficient of 0.5. Each agent in the experiments have a same structure of the actor-critic network, i.e, 4 layers of actor and 4 layers of critic, and each layer has 64 neurons.

As for the hyperparameter settings of MPD and MDPS, the learning rate of the auto-encoder is set as $3 \times 10^{-4}$, the batch size is set as 128, and the KL loss weight set as 0.01. We assume the prior distribution of the latent variable is a 10-dimensional Gaussian distribution. In the baseline SePS, we set hyperparameters according to [4].

In the experiments conducted on harder multi-agent spread tasks, the fusion threshold is set as 1.0, and we compute policy distance matrices and adjust parameter sharing among agents every 2000 steps, using only 100 steps of data for training the auto-encoder and calculation.

In the experiments related to super-hard tasks in SMAC, the fusion threshold is set as 0.5, and we compute customized policy distance matrices and adjust parameter sharing among agents every 20000 steps, using only 500 steps of data for training the auto-encoder and calculation. The customized feature in computing customized policy distances is the "killing reward" from the environment.

All our experiments are carried out on NVIDIA A6000 GPUs. And the experimental results in multi-agent spread tasks and SMAC tasks are demonstrated in Fig. 3 and Fig. 4, respectively.

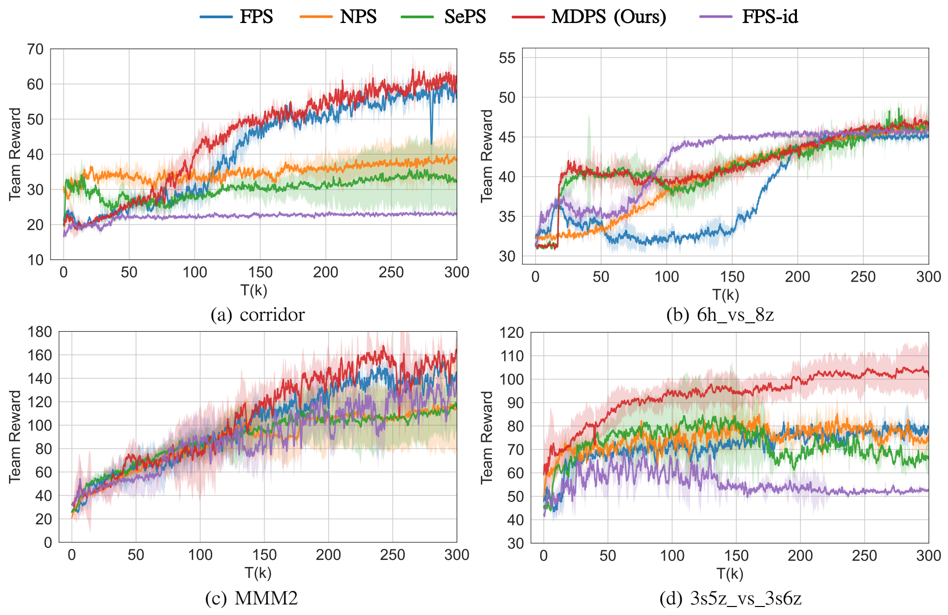


**Figure 4: Comparisons between MDPS and baselines in 4 super-hard tasks in SMAC.**
